# Supplementary material for: Embodied Robot Manipulation in the Era of Foundation Models: Planning and Learning Perspectives
Source: arXiv:2512.22983 source file (2026-08-15)
Supplement: Supplementary file 3 [file 11-appendix_old.tex]

% \clearpage

\appendix

% ---------- Grasping Datasets ----------
\subsection{Details of Grasping Datasets}
\label{appendix: details_grasping_datasets}

\noindent \textbf{Cornell Grasping Dataset}~\cite{jiang2011efficient} consists of 885 RGB-D images capturing 240 different real-world objects, annotated with a total of 8,019 manually labeled grasp rectangles.

\noindent \textbf{Jacquard Dataset}~\cite{depierre2018jacquard} contains 54 thousand RGB-D images of 11 thousand unique objects, with over 1.1 million automatically generated grasp annotations. It leverages a simulation-based pipeline to render synthetic scenes from CAD models and generate ground-truth grasp labels.

\noindent \textbf{GraspNet}~\cite{fang2020graspnet} consists of 97,280 RGB-D images captured from diverse viewpoints across more than 190 cluttered scenes. The dataset includes accurate 3D mesh models for all 88 objects. Each scene is densely annotated with both 6D object poses and corresponding grasp poses, resulting in over 1 billion grasp annotations in total.

\noindent \textbf{ReGrad}~\cite{zhang2022regrad} is built upon the widely used ShapeNet dataset, encompassing 55 object categories and 50,000 distinct objects. It contains 1,020 RGB-D images and over 100 million annotated grasp poses.

\noindent \textbf{ACRONYM}~\cite{eppner2021acronym} contains 17.7 million parallel-jaw grasps across 8,872 objects from 262 distinct categories, each annotated with grasp outcomes obtained from a physics-based simulator.

\noindent \textbf{MetaGraspNet}~\cite{gilles2022metagraspnet} consists of 217k RGB-D images spanning 82 distinct object categories. It provides comprehensive annotations for object detection, amodal perception, keypoint detection, manipulation order, and ambidextrous grasping using both parallel-jaw and vacuum grippers. In addition, it includes a real-world dataset of over 2.3k high-quality, fully annotated RGB-D images, categorized into five levels of difficulty along with an unseen object split to facilitate evaluation under diverse object and layout conditions.
\textbf{MetaGraspNet-V2}~\cite{gilles2023metagraspnetv2} extends the original MetaGraspNet by incorporating a larger number of samples and a broader set of grasp annotations.

\noindent \textbf{Grasp-Anything}~\cite{vuong2024grasp} comprises over 1 million samples accompanied by text descriptions and more than 3 million distinct objects, with approximately 600 million automatically generated grasp rectangles. The dataset is constructed by first performing prompt engineering to create diverse scene descriptions, followed by the use of foundation models to synthesize corresponding images. Grasp poses are then automatically generated and evaluated through a simulation-based pipeline.

\noindent \textbf{Grasp-Anything++}~\cite{vuong2024language} extends the original Grasp-Anything dataset into a large-scale benchmark comprising 1 million images and 10 million grasp-related prompts, specifically designed for language-driven grasp detection tasks.

\noindent \textbf{Grasp-Anything-6D}~\cite{nguyen2024graspanything6d} builds upon Grasp-Anything by providing 1 million point cloud scenes paired with rich language prompts and 200 million high-quality, densely annotated 6-DoF grasp poses. The dataset leverages depth estimation techniques to generate depth maps from RGB images, enabling the reconstruction of detailed 3D scenes for 6-DoF grasp generation.

\noindent \textbf{GraspClutter6D}~\cite{nguyen2024language} provides comprehensive coverage of 200 objects across 75 environmental configurations, including bins, shelves, and tables. The dataset is captured using four RGB-D cameras from multiple viewpoints, resulting in 52,000 RGB-D images. It includes rich annotations with 736,000 6D object poses and 9.3 billion feasible robotic grasps, offering a large-scale benchmark for 6-DoF grasping in cluttered scenes.


% ---------- Manipulation Simulator and Benchmarks for Robot Arm ----------
\subsection{Details of Single-Embodiment Manipulation Simulator and Benchmarks}
\label{appendix: details_of_single-embodiment_benchmarks}

\subsubsection{Common Manipulation Benchmarks} 

We provide a detailed introduction to these benchmarks as follows.

\noindent \textbf{Meta-World}~\cite{yu2020meta} is a MuJoCo-based benchmark featuring a 7-DoF Sawyer arm and 50 diverse tabletop manipulation tasks. It is designed to evaluate meta-reinforcement learning and multi-task learning using low-dimensional proprioceptive inputs. Tasks include picking, opening, and other common single-arm operations.

\noindent \textbf{Franka Kitchen}~\cite{gupta2020relay} is a MuJoCo-based benchmark designed for goal-conditioned reinforcement learning in manipulation scenarios. It features a 7-DoF Franka Panda arm operating in a realistic kitchen environment with common household objects, including a microwave, kettle, overhead light, cabinets, and oven. The benchmark comprises 7 tasks, such as turning the oven knob and opening the sliding cabinet.

\noindent \textbf{RLBench}~\cite{james2020rlbench} features 100 unique, hand-designed tasks with varying difficulty, ranging from simple motions like reaching and door opening to long-horizon, multi-stage tasks such as opening an oven and placing a tray inside. It provides both proprioceptive and visual observations, including RGB, depth, and segmentation masks from an over-the-shoulder stereo camera and an eye-in-hand monocular camera.

\noindent \textbf{CALVIN}~\cite{mees2022calvin} is a PyBullet-based benchmark designed for long-horizon, language-conditioned manipulation. It features a 7-DoF Franka Panda arm operating in four structurally similar but visually distinct tabletop environments, each containing interactive elements such as a sliding door, drawer, button, and switch, along with three colored blocks. The benchmark emphasizes generalization across environment variations and collects 24 hours of demonstration data paired with natural language instructions for long-horizon manipulation tasks.

\noindent \textbf{Robomimic}~\cite{mandlekar2022matters} is a MuJoCo-based benchmark and framework designed to facilitate research in learning from demonstrations for robotic manipulation. It provides a suite of 8 manipulation tasks using a 7-DoF Franka Panda arm, along with over 6,000 human and robot-collected demonstrations across multiple data collection modalities.

\noindent \textbf{ManiSkill}~\cite{mu2maniskill} is a large-scale benchmark for learning manipulation skills from 3D visual inputs, featuring 4 tasks and 162 articulated objects with diverse geometries. Built on SAPIEN, it provides over 36,000 RGB-D and point cloud demonstrations and supports reinforcement learning in physically realistic environments.
\textbf{ManiSkill2} extends ManiSkill with 20 task families, 2,000+ objects, and 4M demonstrations across rigid/soft-body, single/dual-arm, and mobile settings. It adds multi-controller support, action space conversion, and real-time soft-body simulation, enabling efficient large-scale training for generalizable manipulation.

\noindent \textbf{VIMA-Bench}~\cite{jiang2022vima} is a multimodal robot learning benchmark based on the Ravens simulator, featuring 17 tasks with language, image, and segmentation prompts. It supports thousands of task variations across 6 categories, with RGB inputs from multiple views and ground-truth annotations. Actions are defined by parameterized primitives, and demonstrations are generated by scripted oracle agents.

\noindent \textbf{ARNOLD}~\cite{gong2023arnold} is a photo-realistic and physically-accurate simulation benchmark built on NVIDIA Isaac Sim. It features a 7-DoF Franka Panda arm, 20 diverse indoor scenes, and 40 objects, supporting rigid-body and fluid simulation with high-fidelity rendering via GPU ray tracing. The environment provides RGB-D inputs from five camera views and simulates fluid dynamics using position-based methods.

\noindent \textbf{LIBERO}~\cite{liu2023libero} is a benchmark for lifelong robot learning, featuring four task suites: SPATIAL, OBJECT, GOAL (each with 10 tasks for disentangled knowledge transfer), and LIBERO-100 (100 tasks with entangled knowledge). Tasks test generalization over spatial relations, object types, and goals, with a focus on multi-task and long-horizon learning.

\noindent \textbf{THE COLOSSEUM}~\cite{pumacay2024colosseum} is a simulation benchmark built on RLBench, featuring 20 manipulation tasks with over 20,000 task instances. Each task includes 14 types of perturbations (e.g., lighting, object color) to induce covariate shifts for testing OOD generalization. Tasks vary in difficulty by horizon length, and actions are based on primitives like pick, place, and turn. The benchmark also supports real-world replication for selected tasks and includes a standardized challenge protocol.

\noindent \textbf{SimplerEnv}~\cite{li2025evaluating} is a suite of open-source simulated environments for evaluating manipulation policies in real-world setups, replicating RT-1 and BridgeData V2 benchmarks. Built with a standard Gym interface, it supports real-to-sim evaluation for policies like RT-1-X and Octo. SimplerEnv shows strong correlation with real-world performance and enables scalable, reproducible, and reliable benchmarking of generalist robot policies under distribution shifts.

\noindent \textbf{GenSim2}~\cite{hua2025gensim2} is a scalable framework for generating diverse, articulated, and long-horizon manipulation tasks and demonstrations. It uses multi-modal language models such as GPT-4V for task generation and verification, and a keypoint-based motion planner for solving contact-rich 6-DoF tasks.

\noindent \textbf{GemBench}~\cite{garcia2025towards} is a vision-and-language robotic manipulation benchmark built on RLBench to evaluate generalization across tasks and object variations. It includes 16 training tasks covering diverse action primitives and 44 testing tasks organized into four levels of generalization: novel placements, novel rigid objects, novel articulated objects, and novel long-horizon tasks.

\noindent \textbf{RoboTwin}~\cite{mu2025robotwin} is a dual-arm robotic manipulation benchmark designed to evaluate coordination, dexterity, and efficiency across diverse tasks in simulation. It provides a flexible API for generating expert data under varying object placements and conditions, along with offline datasets for each task to support imitation learning and benchmarking. Real-world data is collected using the AgileX Cobot Magic 7 platform with dual arms and RGB-D cameras, offering synchronized multimodal data for both simulation and sim-to-real research.
\textbf{RoboTwin 2.0}~\cite{chen2025robotwin} significantly improves upon RoboTwin 1 by expanding the scale, diversity, and generalization capabilities. It introduces 50 standardized tasks, 731 objects across 147 categories, and 100K expert demonstrations. It also supports multiple robot platforms (e.g., Aloha-AgileX, ARX‑X5, Franka, UR5) and bimanual manipulation. The benchmark integrates multimodal LLM-driven task generation and strong domain randomization to better support generalization and sim-to-real transfer.

\noindent \textbf{GENMANIP}~\cite{gao2025genmanip} is a large-scale tabletop simulation platform for evaluating generalist robots, featuring a structured, LLM-compatible task representation called the Task-oriented Scene Graph (ToSG). ToSG enables diverse task generation, controlled scene layout, and systematic success evaluation. Built on this, GENMANIP-BENCH provides 200 curated scenarios to benchmark generalization across object properties, spatial reasoning, common-sense knowledge, and long-horizon task execution.

\noindent \textbf{VLABench}~\cite{zhang2024vlabench} is a Mujoco-based open-source benchmark for evaluating foundation-model-driven, language-conditioned robotic manipulation. It features 100 tasks (60 primitive, 40 composite) across 2,000+ 3D assets and supports diverse skill assessment, including tool use, pouring, and long-horizon reasoning. Built with modular scenes and rich visual-linguistic prompts, it uses a 7-DoF Franka Panda robot and supports multiple embodiments. The benchmark emphasizes real-world relevance, generalization, and broad task diversity.

\noindent \textbf{AGNOSTOS}~\cite{zhou2025agnostos} is a benchmark on RLBench for evaluating zero-shot cross-task generalization of vision-language-action models. It includes 18 training tasks and 23 unseen test tasks with varying difficulty. Models are evaluated across foundation, human-video-pretrained, and in-domain types under a standardized protocol, enabling fair comparison of generalization capabilities beyond seen tasks.

\noindent \textbf{ROBOEVAL}~\cite{wang2025roboeval} is a benchmark for bimanual manipulation across service, warehouse, and industrial tasks. It includes 8 tasks, 3,000+ human demonstrations with varied contexts, and offers fine-grained metrics to support imitation learning and demonstration-driven policy evaluation.

\noindent \textbf{INT-ACT}~\cite{fang2025intention} builds upon the SimplerEnv benchmark, significantly expanding its scope from 4 to 50 tasks based on the BridgeV2 dataset. It introduces an additional metric to track policy intention and organizes tasks into three categories: object diversity, language complexity, and vision language reasoning. INT-ACT aims to comprehensively evaluate the generalization abilities of VLAs in simulation.

\noindent \textbf{TacSL}~\cite{yu2020meta} is a GPU-accelerated tactile simulation module for visuotactile sensors, integrated into a general-purpose robotics simulator. It simulates physical interactions and computes tactile RGB images and force fields, both optimized via GPU parallelization for speed and stability. TacSL also includes tools to support efficient tactile policy learning and demonstrates effective sim-to-real transfer.

\noindent \textbf{ManiFeel}~\cite{yu2020meta} is a scalable visuotactile simulation benchmark for supervised policy learning. It offers (1) a diverse suite of contact-rich tasks and human demonstrations to evaluate tactile feedback's role in multimodal learning; (2) a modular policy architecture design that separates sensing, representation, and control for flexible experimentation; (3) comprehensive empirical analysis across simulation and real-world settings; and (4) validated sim-to-real consistency, supporting reproducible tactile policy research.


\subsubsection{Deformable Object Manipulation Benchmarks}
We provide a detailed introduction to these benchmarks as follows.

\noindent \textbf{SoftGym}~\cite{lin2021softgym} is a benchmark suite for manipulating deformable objects such as ropes, cloths, and fluids. It is divided into three components: SoftGym-Medium, SoftGym-Hard, and SoftGym-Robot. SoftGym-Medium and SoftGym-Hard feature tasks that utilize an abstract action space, with the latter offering four more challenging scenarios. In contrast, SoftGym-Robot includes tasks where actions are executed through a Sawyer or Franka robotic arm, enabling more realistic robot-based manipulation.

\noindent \textbf{PlasticineLab}~\cite{huang2021plasticinelab} is a suite of challenging soft-body manipulation tasks built upon a differentiable physics simulator. In these tasks, agents are required to deform one or more 3D plasticine objects using rigid-body manipulators. The simulator enables the execution of complex soft-body operations such as pinching, rolling, chopping, molding, and carving, providing a rich and versatile environment for studying deformable object manipulation.


\subsubsection{Mobile Manipulation Benchmarks}
We provide a detailed introduction to these benchmarks as follows.

\noindent \textbf{ManipulaTHOR}~\cite{ehsani2021manipulathor} is an extension of the AI2-THOR framework that equips agents with a simplified 3-DoF robotic arm and a spherical grasper for low-level object manipulation. Built on Unity and NVIDIA’s PhysX, it supports realistic physics, diverse indoor scenes, and articulated objects. The arm can be controlled via forward or inverse kinematics, enabling actions such as wrist positioning, object picking, and releasing. The grasper abstracts grasping as sphere-object collisions to simplify manipulation research. ManipulaTHOR supports multi-modal sensing (RGB, depth, position) and achieves a simulation speed of 300 FPS, enabling efficient large-scale training.

\noindent \textbf{HomeRobot}~\cite{yenamandra2023homerobot} is introduced as a core task for in-home robotics, accompanied by the first reproducible benchmark for evaluating end-to-end mobile manipulation systems in both simulation and real-world settings. The benchmark features a mix of seen and unseen object categories and supports arbitrary object sets, allowing for deployment in diverse, real-world environments. In simulation, OVMM utilizes 200 human-authored interactive 3D scenes within AI Habitat. For real-world evaluation, it employs the Hello Robot Stretch platform in a controlled apartment setting. The benchmark is integrated with HomeRobot, a unified software framework offering consistent APIs across simulation and real-world platforms, supporting tasks such as manipulation, navigation, and continual learning.

\noindent \textbf{BEHAVIOR-1K}~\cite{li2023behavior} is a large-scale benchmark featuring 1,000 everyday household activities within realistic, interactive environments. It consists of two main components: the BEHAVIOR-1K Dataset, which defines each activity using predicate logic and includes 50 richly annotated scenes and over 5,000 3D object models; and OMNIGIBSON, a physics-based simulation environment built on NVIDIA Omniverse and PhysX 5. OMNIGIBSON supports the simulation of rigid, deformable, and fluid objects, along with dynamic object states such as temperature, soakedness, and dirtiness. Together, these components enable diverse, high-fidelity activity simulations for advancing embodied AI research.


\subsubsection{Humanoid Manipulation Benchmarks}

We provide a detailed introduction to these benchmarks as follows.

\noindent \textbf{BiGym}~\cite{chernyadev2025bigym} is a demonstration-driven benchmark for mobile bimanual manipulation using a humanoid robot embodiment. It includes 40 visually diverse tasks, ranging from simple object transport to interactions with articulated appliances such as dishwashers. Unlike prior humanoid benchmarks that rely on dense reward reinforcement learning, BiGym uses sparse rewards and provides 50 human-collected multimodal demonstrations per task, enabling evaluation of both imitation learning and reinforcement learning. It supports two action modes: a whole-body mode that includes locomotion and manipulation, and a bimanual mode that focuses on upper-body manipulation with a fixed lower body. Built on MuJoCo and based on the Unitree H1 robot equipped with Robotiq grippers, BiGym offers a realistic and flexible testbed for advancing research in mobile humanoid manipulation.

\noindent \textbf{HumanoidBench}~\cite{sferrazza2024humanoidbench} is a simulation benchmark designed to advance learning and control algorithms for humanoid robots, which face challenges in real-world deployment due to their complex form factors and hardware constraints. The benchmark includes 27 tasks: 12 focused on locomotion and 15 on whole-body manipulation. Locomotion tasks provide simpler settings for humanoid control, while manipulation tasks require full-body coordination to solve complex, practical scenarios such as truck unloading and shelf rearrangement. With up to 61 actuators per agent, HumanoidBench offers a rich testbed for evaluating high-dimensional control and coordination strategies in simulation.

\noindent \textbf{HumanoidGen}~\cite{jing2025humanoidgen} is an LLM-driven framework for generating diverse humanoid manipulation tasks and collecting large-scale demonstrations. It uses an LLM planner to create environment setups and success conditions from language prompts and 3D assets. Tasks are decomposed into atomic hand operations with spatial constraints, which are translated into code-based constraints and solved via trajectory optimization. To handle complex long-horizon tasks, a Monte Carlo Tree Search (MCTS) module enhances test-time reasoning. Built on this framework, HGen-Bench introduces 20 bimanual manipulation tasks for the Unitree H1-2 robot with Inspire hands, using SAPIEN for simulation. Experimental results show MCTS improves constraint satisfaction and policy performance improves steadily with more demonstrations.


% ---------- Cross-Embodiment Manipulation Simulator and Benchmarks ----------
\subsection{Details of Cross-Embodiment Manipulation Simulator and Benchmarks}
\label{appendix: details_of_cross-embodiment_benchmarks}

\noindent \textbf{RoboSuite}~\cite{zhu2020robosuite} is a modular and extensible simulation framework built on MuJoCo, designed for robot learning. It supports over 10 robot models, 9 grippers, and various bases and controllers with realistic physical parameters. Its plug-and-play architecture allows flexible combinations of embodiments, and each robot instance manages its own initialization and control

\noindent \textbf{CortexBench}~\cite{majumdar2023we} is a comprehensive benchmark designed to evaluate pre-trained visual representations (PVRs) across diverse embodied AI (EAI) tasks. It includes 17 tasks from 7 established benchmarks, covering a range of domains such as dexterous and tabletop manipulation (Adroit~\cite{rajeswaran2018learning}, MetaWorld~\cite{yu2020meta}, TriFinger~\cite{wuthrich2021trifinger}). Each task uses standardized policy learning paradigms (e.g., IL and RL) to isolate the effect of visual representations. By unifying these tasks, CORTEXBENCH enables large-scale, systematic evaluation of PVRs toward building an artificial visual cortex for embodied intelligence.

\noindent \textbf{ORBIT}~\cite{mittal2023orbit}, later renamed Isaac Lab, is a unified and modular simulation framework for robot learning, built on NVIDIA Isaac Sim. It enables efficient creation of photorealistic environments with high-fidelity simulation of both rigid and deformable body dynamics. The framework offers a diverse suite of over 20 benchmark tasks, ranging from simple cabinet opening to complex multi-stage room reorganization. It includes 16 robotic platforms, 4 sensor modalities, and 10 motion generators, allowing flexible configurations for both fixed-base and mobile manipulators. Leveraging GPU-accelerated parallelization, Isaac Lab supports fast reinforcement learning and large-scale demonstration collection. It is designed to support reinforcement learning, imitation learning, representation learning, and task and motion planning, with modular components that promote extensibility and interdisciplinary research.

\noindent \textbf{RoboCasa}~\cite{nasiriany2024robocasa} is a large-scale simulation benchmark built on top of RoboSuite to support household manipulation tasks in room-scale environments. It features mobile manipulators, humanoids, and quadrupeds, and integrates photorealistic rendering via NVIDIA Omniverse. RoboCasa defines 25 atomic tasks based on eight core sensorimotor skills (e.g., pick-and-place, button press, navigation) and 75 composite tasks generated using LLMs, covering realistic household activities like cooking and cleaning. Demonstrations are collected via human teleoperation and scaled up using MimicGen, which synthesizes new trajectories by adapting object-centric segments.

\noindent \textbf{Genesis}~\cite{genesis2024genesis} is a high-performance, general-purpose physics simulation platform for Robotics, Embodied AI, and Physical AI. It combines a re-engineered universal physics engine with ultra-fast simulation, photorealistic rendering, and modular generative data tools. Genesis supports diverse physics solvers (rigid, deformable, fluids, etc.), a wide range of material types, and various robot embodiments. It is cross-platform, highly extensible, differentiable, and designed for ease of use, aiming to unify physics simulation and automate data generation for scalable embodied intelligence research.

\noindent \textbf{ManiSkill3}~\cite{tao2025maniskill3} significantly improves over ManiSkill2 by enabling high-speed GPU-parallelized simulation (30,000+ FPS) with low memory usage, expanding to 12 environment types and 20+ robot embodiments, and supporting heterogeneous simulations across parallel environments. It offers a unified, user-friendly API with rich tools for task creation, domain randomization, and trajectory replay. Additionally, it introduces a scalable pipeline to generate large datasets from few demonstrations using imitation learning, making it a more efficient and versatile platform for generalizable robot learning.

\noindent \textbf{RoboVerse}~\cite{geng2025roboverse} is a unified simulation platform built on METASIM, which enables scalable robot learning through cross-simulator integration, hybrid simulation, and cross-embodiment transfer. By standardizing environment configuration, interfaces, and APIs, it allows seamless switching between simulators, combining their strengths (e.g., MuJoCo physics with Isaac Sim rendering), and reusing trajectories across different robot types, making it a flexible and powerful tool for general-purpose robotic benchmarks.

\noindent \textbf{VIKI-Bench}~\cite{kang2025viki} is a large-scale benchmark for embodied multi-agent collaboration, featuring over 20,000 task instances across 100 diverse scenes built on RoboCasa and ManiSkill3. It includes six types of heterogeneous agents such as humanoids, wheeled arms, and quadrupeds, interacting with more than 1,000 unique object combinations. Tasks are organized into three levels: Agent Activation, Task Planning, and Trajectory Perception. Each scene provides both global and egocentric visual inputs to support perception and planning. The accompanying VIKI-R framework enhances reasoning capabilities through Chain-of-Thought prompting and reinforcement learning, showing strong performance across all task levels.


% ---------- Trajectory Datasets ----------
\subsection{Details of Trajectory Datasets}
\label{appendix: details_of_trajectory_datasets}

\noindent \textbf{MIME}~\cite{sharma2018multiple} is a human-robot demonstration dataset designed to enable learning of complex manipulation tasks that cannot be solved by self-supervision alone. It includes 8,260 kinesthetic demonstrations paired with corresponding human-performed videos, covering over 20 tasks from simple pushing to challenging object stacking. Demonstrations are collected from multiple trained human operators to ensure diversity and scalability, using both kinesthetic teaching and visual demonstration for richer supervision.

\noindent \textbf{BridgeData}~\cite{ebert2021bridge} is a large-scale collection of 7,200 demonstrations across 71 kitchen-related tasks in 10 miniature kitchen environments, using a low-cost 6-DoF WidowX250s robot. Demonstrations are collected via human teleoperation using an Oculus Quest and multiple RGB or RGB-D cameras. The dataset features randomized environments and camera setups to improve diversity and generalization, aiming to support reproducible and accessible real-world robotic learning. 
\noindent \textbf{BridgeData V2}~\cite{walke2023bridgedata} is a large-scale, multi-task robot manipulation dataset designed to support generalizable skill learning. It contains over 60,000 trajectories (50,365 expert and 9,731 scripted) spanning 13 diverse skills (e.g., pick-and-place, folding, door opening) across 24 environments with 100+ objects. Data was collected using low-cost hardware in varied, randomized scenes without per-trajectory resets or task labels. Task annotations were added via crowdsourcing. The dataset emphasizes task diversity, environmental variation, and includes both human and autonomous demonstrations for flexibility in training paradigms.

\noindent \textbf{BC-Z}~\cite{jang2022bc} collects large-scale collection of 25,877 robot demonstrations across 100 diverse manipulation tasks, acquired using a shared autonomy setup where human operators can intervene during policy rollouts. Demonstrations were collected via Oculus-based teleoperation across 12 robots and 7 operators, combining expert-only and human-guided correction (HG-DAgger) phases. Additionally, 18,726 human videos of the same tasks were collected for cross-modal learning. The system enables zero-shot and few-shot generalization to unseen tasks and supports asynchronous closed-loop visuomotor control at 10Hz.

\noindent \textbf{RT-1}~\cite{brohan2023rt} collects a large-scale robotic dataset and system designed to enable generalization across diverse manipulation tasks. Collected over 17 months using 13 mobile manipulators, it comprises 130k demonstrations covering 700+ language instructions across varied office kitchen environments. Each instruction is labeled with verb-noun phrases (e.g., “pick apple”) and grouped into skills. The data includes a wide range of tasks, objects, and scenes to support robust policy learning. The goal is to build a general robot policy that performs well on seen and unseen tasks, with strong transfer and generalization capabilities.

\noindent \textbf{RH20T}~\cite{fang2023rh20t} is a large-scale, diverse, and multimodal robot manipulation dataset designed to support general-purpose manipulation learning. It contains over 110,000 robot trajectories and an equal number of human demonstrations, covering 147 tasks and 42 manipulation skills using 7 robot configurations (multiple arms, grippers, sensors). It features multi-sensor data (RGB, depth, force-torque, tactile, audio, proprioception), and supports dense human-robot pairing with a hierarchical data structure. Tasks include both atomic and compositional sequences, and data is collected via intuitive haptic teleoperation. RH20T emphasizes diversity, scale, multimodality, and semantic richness for complex contact-rich manipulations.

\noindent \textbf{RoboSet}~\cite{bharadhwaj2024roboagent} is a compact yet diverse real-world robot manipulation dataset comprising 7,500 human-teleoperated trajectories across 12 core skills (e.g., wiping, sliding, opening/closing objects). Tasks are structured around meaningful household activities and instantiated in four kitchen scenes with varied objects and layouts, promoting compositionality and generalization. To enhance robustness to out-of-distribution scenarios, RoboSet introduces a fully automated semantic augmentation pipeline that generates diverse variations of each trajectory via frame-wise inpainting, guided by text prompts and masks from the Segment Anything model.

\noindent \textbf{Open X-Embodiment}~\cite{o2024open} is a large-scale, unified robot manipulation dataset comprising over 1 million real-world trajectories across 22 robot embodiments, including single-arm robots, bi-manual systems, and quadrupeds. It aggregates 60 datasets from 34 research labs, standardized in the RLDS format (tfrecord), enabling compatibility with diverse action spaces and modalities (e.g., RGB, depth, point cloud) and efficient loading in major deep learning frameworks. The dataset features rich language annotations, enabling skill and object diversity analysis. While many tasks involve pick-and-place, the long-tail includes behaviors like wiping and assembling, covering a broad range of everyday household objects and scenes.

\noindent \textbf{DROID}~\cite{khazatsky2024droid} is a large-scale, diverse robot manipulation dataset featuring 76,000 successful trajectories collected across 13 institutions, 52 buildings, and 564 unique real-world scenes using a standardized mobile Franka Panda platform. It supports rich multimodal data (RGB, joint states, control actions, language) and was collected via teleoperation using Meta Quest 2 controllers, guided by a shared protocol to ensure consistency and diversity. DROID emphasizes diversity across tasks, objects, scenes, viewpoints, and interaction locations, enabling robust generalization. Each trajectory is annotated with natural language instructions, and the dataset includes post-hoc calibration and quality-checked camera parameters to support 3D perception and policy learning.

\noindent \textbf{ARIO}~\cite{wang2024all} is a large-scale multimodal dataset designed to support general-purpose embodied intelligence across diverse tasks, robots, and environments. It includes over 3 million episodes and 321,000 tasks, integrating data from real-world collection, simulation, and transformed open-source datasets. ARIO supports five sensory modalities—vision (2D/3D), sound, text, proprioception, and tactile—with temporally aligned recordings across modalities. Real-world data was collected using platforms like Cobot Magic and Cloud Ginger XR-1, featuring bimanual, contact-rich, deformable, and human-robot collaboration tasks, while simulation data comes from Habitat, MuJoCo, and SeaWave. Additionally, ARIO standardizes and unifies diverse datasets like Open X-Embodiment, RH20T, and ManiWAV, the latter introducing audio for multimodal reasoning. The dataset's rich diversity in skills, scenes, robot morphologies, and modalities makes it a comprehensive resource for advancing cross-embodiment and generalizable robot learning.

\noindent \textbf{RoboMIND}~\cite{wu2024robomind} is a large-scale, standardized dataset designed for diverse and complex robot manipulation tasks across multiple embodiments, including single-arm, dual-arm, and humanoid robots. It features over 479 distinct tasks and supports long-horizon, coordinated, precision, and scene-understanding skills, collected via teleoperation using VR, 3D-printed interfaces, and motion capture suits. With more than 96 object categories across five real-world usage domains and fine-grained linguistic annotations, RoboMIND offers temporally aligned multimodal data (RGB-D, proprioception, tactile) in a unified H5 format. Its consistent data collection protocol and rich embodiment-task diversity make it ideal for training and evaluating generalizable, cross-embodiment robotic policies.

\noindent \textbf{RoboFAC}~\cite{lu2025robofac} is a failure-centric robotic manipulation dataset featuring 14 simulated and 6 real-world tasks, including 2 real-world–only tasks, designed to support both short- and long-horizon tasks in dynamic environments. It includes over 9,000 failure trajectories and 1,280 successful ones, with diverse camera viewpoints and backgrounds to enhance visual generalization. Failures are categorized across three hierarchical levels and annotated with rich textual descriptions. The dataset comprises 78K video QA samples across eight question types, enabling comprehensive evaluation of task understanding, failure analysis, and correction reasoning. Annotations combine manual inspection and GPT-4o–assisted generation for high-quality QA benchmarking.


% ---------- Embodied QA and Affordance Datasets ----------
\subsection{Details of Embodied QA and Affordance Datasets}
\label{appendix: details_of_embodied_qa_and_affordance_datasets}

\noindent \textbf{OpenEQA}~\cite{majumdar2024openeqa} is a large-scale open-vocabulary benchmark for Embodied Question Answering (EQA) that supports two settings: episodic-memory QA (EM-EQA) and active exploration QA (A-EQA). It contains over 1600 human-annotated questions across 180+ real-world environments using RGB-D videos and 3D scans from datasets like ScanNet and HM3D. Questions span seven categories, including object recognition, spatial reasoning, functional reasoning, and object localization. Unlike previous EQA benchmarks, OpenEQA features open-ended language, realistic scenes, and LLM-based evaluation, making it a challenging and practical benchmark for testing embodied agents and vision-language models.

\noindent \textbf{ManipVQA}~\cite{huang2024manipvqa} is a large-scale visual question answering benchmark designed to evaluate vision-language models on robotic manipulation tasks grounded in affordance understanding and physical reasoning. It includes over 80K samples spanning four task types: object-level visual reasoning, affordance recognition, affordance grounding, and physical concept understanding (e.g., liquid containment, transparency). ManipVQA integrates diverse data sources, including real-world and simulated datasets like HANDAL, PartAfford, PhysObjects, and PACO, and uses referring expression comprehension/generation (REC/REG) formats to localize or describe regions of interest. It emphasizes fine-grained functional perception critical for manipulation, making it a targeted benchmark for robotics-centric multimodal learning.

\noindent \textbf{ManipBench}~\cite{zhao2025manipbench} is a multiple-choice VQA benchmark for robotic manipulation, featuring 12,617 questions generated from three data sources: public robotic datasets, in-house fabric manipulation setups, and simulation environments. It focuses on evaluating visual language models (VLMs) through keypoint prediction and trajectory understanding across diverse manipulation tasks. Questions are constructed using image annotations, sampled interaction points, and task descriptions. The benchmark assesses model accuracy and generalization with both VLM and human evaluations, and further validates performance through real-world robot experiments on unseen tasks.

\noindent \textbf{PointArena}~\cite{cheng2025pointarena} is an evaluation suite for fine-grained spatial grounding, formulated as a language-conditioned pointing task. It includes three components: \textit{Point-Bench}, a curated benchmark of 982 text-image pairs with pixel-level masks across five categories (spatial, affordance, counting, steerable, and reasoning); \textit{Point-Battle}, a live human preference-based model comparison arena; and \textit{Point-Act}, a real-world robotic pointing task. Unlike prior benchmarks that focus on classification or captioning, PointArena emphasizes precise localization from natural language, offering a unified framework to assess MLLMs' ability to bridge language, vision, and physical action.

\noindent \textbf{Robo2VLM}~\cite{chen2025robo2vlm} is a large-scale benchmark for manipulation-aware VQA, generated from real-world human-teleoperated robot trajectories in the Open X-Embodiment (OXE) dataset. It produces over 3 million multiple-choice VQA samples, covering 463 scenes, 3,396 manipulation tasks, and 149 manipulation skills. Questions are grounded in synchronized multi-modal data (e.g., RGB, depth, force, and gripper state) and span three reasoning categories: spatial reasoning, interaction reasoning, and goal-conditioned reasoning. By segmenting long-horizon trajectories into semantic phases (e.g., approach, contact, release), Robo2VLM enables precise and phase-aware question generation, offering a high-quality, scalable benchmark to evaluate vision-language models in real-world robot manipulation settings.

\noindent \textbf{PAC Bench}~\cite{gundawar2025pac} is a diagnostic benchmark for assessing a VLM’s physical reasoning capabilities relevant to robotic manipulation. It focuses on three foundational aspects—Properties, Affordances, and Constraints—that collectively determine action feasibility. PAC Bench includes thousands of curated real and simulated scenes with fine-grained annotations, testing a model’s ability to infer material traits, actionable potentials, and physical limitations of objects. By targeting these core concepts, PAC Bench provides a rigorous and interpretable framework for evaluating manipulation-centric reasoning, without requiring access to a specific robot or environment.
