# Supplementary material for: Embodied Robot Manipulation in the Era of Foundation Models: Planning and Learning Perspectives
Source: arXiv:2512.22983 source file (2026-08-15)
Supplement: Supplementary file 4 [file ablation_action_horizon.tex]

\begin{table}[t]
\centering
\caption{Controlled comparison of action-chunk horizons. Action Chunk $H$ denotes jointly predicting a sequence of $H$ future actions. LIBERO reports the success rate on the original Spatial suite, while LIBERO-plus reports the average success rate across its perturbation settings. Compared with single-step prediction, both multi-step variants improve performance. However, the preferred horizon is evaluation-dependent: horizon 4 performs best on LIBERO, whereas horizon 8 achieves the highest robustness on LIBERO-plus. All values are success rates (\%)~\cite{wu2026vlanext}.}
\label{tab:abla_action_chunk}
\small
\setlength{\tabcolsep}{8pt}
\begin{tabular}{lcc}
\toprule
\textbf{Action horizon} &
\textbf{LIBERO} &
\textbf{LIBERO-plus} \\
\midrule
Action Chunk 1 & 64.4 & 34.0 \\
Action Chunk 4 & \textbf{75.4} & 40.0 \\
Action Chunk 8 & 74.6 & \textbf{43.4} \\
\bottomrule
\end{tabular}
\end{table}
