# Supplementary material for: Embodied Robot Manipulation in the Era of Foundation Models: Planning and Learning Perspectives
Source: arXiv:2512.22983 source file (2026-08-15)
Supplement: Supplementary file 5 [file ablation_arch.tex]

\begin{table*}[htbp]
\centering
\caption{Controlled evidence on policy-module capacity, VLM--policy coupling, and history aggregation. Results are compared only within each experimental block. LIBERO and LIBERO-plus report success rates (\%), while CALVIN reports the average number of consecutively completed tasks.}
\label{tab:abla_arch}
\small
\begin{tabular}{llcc}
\toprule
\textbf{Controlled factor} & \textbf{Variant} & \textbf{Primary benchmark} & \textbf{Result} \\
\midrule
\multirow{3}{*}{Policy-module capacity~\cite{wu2026vlanext}}
& RT-2-like action-token baseline & LIBERO & 19.8 \\
& Separate policy head & LIBERO & 30.2 \\
& Large dedicated policy module & LIBERO & \textbf{64.4} \\
\midrule
\multirow{2}{*}{VLM--policy coupling~\cite{wu2026vlanext}}
& Loose connection & LIBERO / LIBERO-plus & \textbf{90.0} / 53.7 \\
& Tight layer-wise connection & LIBERO / LIBERO-plus & \textbf{90.0} / \textbf{55.4} \\
\bottomrule
\end{tabular}
\end{table*}
